# Supplementary material for: Hot super-Earths stripped by their host stars
Source: arXiv:1604.05220 source file (2016-04-18)
Supplement: Supplementary file 1 [file Supplementary_information.pdf]

**Supplementary Information: Hot super-Earths stripped by their host stars , M. S. Lundkvist et al.**

**Supplementary Table 1: Parameters for the 102 host stars with detected oscillations.**

| KIC number | $\Delta\nu$ ( $\mu\text{Hz}$ ) | $\sigma(\Delta\nu)$ ( $\mu\text{Hz}$ ) | $T_{\text{eff}}$ (K) | $\sigma(T_{\text{eff}})$ (K) | [Fe/H] (dex) | $\sigma([\text{Fe}/\text{H}])$ (dex) | Ref. |
|------------|--------------------------------|----------------------------------------|----------------------|------------------------------|--------------|--------------------------------------|------|
| 3102384    | 124.7                          | 0.4                                    | 5739                 | 75                           | 0.35         | 0.1                                  | 1    |
| 3425851    | 93.0                           | 0.5                                    | 6343                 | 85                           | -0.04        | 0.1                                  | 1    |
| 3531558    | 86.8                           | 0.3                                    | 5747                 | 85                           | 0.03         | 0.1                                  | 1    |
| 3544595    | 145.8                          | 0.4                                    | 5669                 | 75                           | -0.18        | 0.1                                  | 1    |
| 3632418    | 60.9                           | 0.6                                    | 6305                 | 50                           | -0.03        | 0.1                                  | 2    |
| 3640905    | 30.7                           | 0.5                                    | 4991                 | 75                           | 0.28         | 0.1                                  | 1    |
| 4141376    | 128.2                          | 0.4                                    | 6134                 | 91                           | -0.24        | 0.1                                  | 1    |
| 4143755    | 77.1                           | 0.3                                    | 5622                 | 106                          | -0.40        | 0.11                                 | 1    |
| 4262040    | 40.8                           | 0.3                                    | 5299                 | 147                          | -0.35        | 0.3                                  | 3    |
| 4349452    | 98.5                           | 0.9                                    | 6270                 | 79                           | -0.04        | 0.1                                  | 1    |
| 4450844    | 72.8                           | 0.4                                    | 5968                 | 59                           | -0.20        | 0.3                                  | 4    |
| 4769799    | 15.3                           | 0.3                                    | 5079                 | 143                          | -0.43        | 0.3                                  | 3    |
| 4815520    | 136.0                          | 0.3                                    | 5755                 | 50                           | 0.20         | 0.08                                 | 5    |
| 4914423    | 82.0                           | 0.4                                    | 5845                 | 88                           | 0.07         | 0.11                                 | 1    |
| 5042210    | 66.7                           | 0.6                                    | 6007                 | 120                          | 0.05         | 0.15                                 | 3    |
| 5088536    | 110.0                          | 0.4                                    | 5884                 | 75                           | 0.00         | 0.25                                 | 1    |
| 5094751    | 90.7                           | 0.4                                    | 5952                 | 75                           | -0.08        | 0.1                                  | 1    |
| 5383248    | 149.4                          | 0.5                                    | 5690                 | 77                           | 0.04         | 0.07                                 | 6    |
| 5511081    | 63.6                           | 0.4                                    | 5923                 | 77                           | -0.07        | 0.1                                  | 1    |
| 5513648    | 76.9                           | 0.3                                    | 5904                 | 85                           | -0.07        | 0.1                                  | 1    |
| 5514383    | 113.3                          | 0.6                                    | 6184                 | 81                           | 0.12         | 0.1                                  | 1    |
| 5561278    | 56.8                           | 0.6                                    | 6081                 | 75                           | -0.03        | 0.1                                  | 1    |
| 5652983    | 29.4                           | 0.3                                    | 5198                 | 95                           | 0.19         | 0.11                                 | 1    |
| 5780885    | 56.4                           | 0.7                                    | 6027                 | 75                           | 0.10         | 0.1                                  | 1    |
| 5866724    | 89.6                           | 0.6                                    | 6169                 | 50                           | 0.09         | 0.08                                 | 1    |
| 5905822    | 82.2                           | 0.4                                    | 6115                 | 165                          | -0.06        | 0.3                                  | 3    |
| 6196457    | 67.1                           | 0.5                                    | 5871                 | 94                           | 0.17         | 0.11                                 | 1    |
| 6268648    | 87.9                           | 0.6                                    | 6044                 | 117                          | -0.24        | 0.11                                 | 1    |
| 6278762    | 179.6                          | 0.5                                    | 5046                 | 74                           | -0.37        | 0.09                                 | 2    |
| 6448890    | 17.4                           | 0.3                                    | 4840                 | 97                           | 0.20         | 0.16                                 | 1    |
| 6521045    | 77.1                           | 0.5                                    | 5825                 | 75                           | 0.02         | 0.1                                  | 1    |
| 6528464    | 75.4                           | 0.4                                    | 5588                 | 99                           | -0.10        | 0.1                                  | 1    |

|         |       |     |      |     |       |      |   |
|---------|-------|-----|------|-----|-------|------|---|
| 6678383 | 56.5  | 0.4 | 5711 | 74  | -0.55 | 0.07 | 7 |
| 7199397 | 38.7  | 0.4 | 5896 | 75  | -0.17 | 0.1  | 1 |
| 7215603 | 83.4  | 0.5 | 6173 | 93  | 0.17  | 0.1  | 1 |
| 7449136 | 77.2  | 0.4 | 6099 | 75  | 0.04  | 0.1  | 1 |
| 7582689 | 70.0  | 0.6 | 6004 | 75  | 0.07  | 0.1  | 8 |
| 7670943 | 88.3  | 0.6 | 6463 | 110 | 0.09  | 0.11 | 1 |
| 7887791 | 156.1 | 0.6 | 5547 | 100 | -0.04 | 0.15 | 8 |
| 7941200 | 130.1 | 0.5 | 5952 | 119 | 0.02  | 0.15 | 3 |
| 8013439 | 86.0  | 0.4 | 6152 | 100 | -0.18 | 0.1  | 7 |
| 8077137 | 69.0  | 0.7 | 6072 | 75  | -0.09 | 0.1  | 1 |
| 8176564 | 77.7  | 0.4 | 6109 | 51  | -0.20 | 0.3  | 4 |
| 8292840 | 93.2  | 0.6 | 6239 | 94  | -0.14 | 0.1  | 1 |
| 8349582 | 83.4  | 0.4 | 5699 | 74  | 0.30  | 0.1  | 1 |
| 8478994 | 178.3 | 0.6 | 5417 | 75  | -0.32 | 0.07 | 1 |
| 8494142 | 62.2  | 0.6 | 6144 | 106 | 0.13  | 0.1  | 1 |
| 8554498 | 62.2  | 0.4 | 5753 | 75  | 0.05  | 0.1  | 1 |
| 8684730 | 52.4  | 0.5 | 5882 | 87  | 0.16  | 0.1  | 1 |
| 8686097 | 103.7 | 0.3 | 5833 | 50  | -0.27 | 0.08 | 5 |
| 8700771 | 69.0  | 0.4 | 5665 | 50  | -0.39 | 0.08 | 5 |
| 8753657 | 121.0 | 0.4 | 5538 | 74  | 0.18  | 0.07 | 7 |
| 8801316 | 57.7  | 0.5 | 6718 | 183 | -0.06 | 0.3  | 3 |
| 8803882 | 25.2  | 0.4 | 5250 | 169 | 0.06  | 0.3  | 3 |
| 8822366 | 71.1  | 0.3 | 6034 | 92  | -0.14 | 0.1  | 1 |
| 8866102 | 94.5  | 0.7 | 6325 | 75  | 0.01  | 0.1  | 1 |
| 8868481 | 40.4  | 0.3 | 5779 | 67  | -0.20 | 0.3  | 4 |
| 9072639 | 85.2  | 0.3 | 6306 | 220 | -0.36 | 0.3  | 3 |
| 9394953 | 65.2  | 0.5 | 6018 | 65  | -0.20 | 0.3  | 4 |
| 9414417 | 59.6  | 0.8 | 6253 | 75  | -0.13 | 0.1  | 1 |
| 9451706 | 95.3  | 0.3 | 6106 | 106 | 0.33  | 0.1  | 1 |
| 9579208 | 61.0  | 0.6 | 6422 | 56  | -0.20 | 0.3  | 4 |
| 9579641 | 131.2 | 0.3 | 6395 | 184 | -0.22 | 0.3  | 3 |
| 9590976 | 72.3  | 0.4 | 6171 | 109 | -0.12 | 0.1  | 7 |
| 9592705 | 53.4  | 0.5 | 6174 | 92  | 0.22  | 0.1  | 1 |
| 9602613 | 129.6 | 0.4 | 5467 | 148 | -0.12 | 0.3  | 3 |
| 9696358 | 50.7  | 0.6 | 6131 | 75  | 0.13  | 0.1  | 1 |
| 9697131 | 59.5  | 0.4 | 6491 | 69  | -0.20 | 0.3  | 4 |
| 9872292 | 65.0  | 0.7 | 6260 | 116 | 0.10  | 0.11 | 1 |

|          |       |     |      |     |       |      |     |
|----------|-------|-----|------|-----|-------|------|-----|
| 9955598  | 153.1 | 0.4 | 5460 | 75  | 0.08  | 0.1  | 1   |
| 10026544 | 26.0  | 0.6 | 6149 | 122 | -0.42 | 0.15 | 3   |
| 10130039 | 143.5 | 0.4 | 5828 | 100 | -0.08 | 0.1  | 7   |
| 10136549 | 55.9  | 0.4 | 5684 | 175 | 0.02  | 0.1  | 7   |
| 10264660 | 54.4  | 0.5 | 6378 | 75  | -0.02 | 0.1  | 1   |
| 10272858 | 22.7  | 0.3 | 5208 | 68  | -0.20 | 0.3  | 4   |
| 10289119 | 37.2  | 0.6 | 6056 | 165 | -0.17 | 0.3  | 3   |
| 10585852 | 23.3  | 0.3 | 5048 | 75  | -0.03 | 0.1  | 1   |
| 10586004 | 69.7  | 0.4 | 5770 | 83  | 0.29  | 0.1  | 1   |
| 10593626 | 165.2 | 0.4 | 5570 | 50  | -0.26 | 0.06 | K15 |
| 10666592 | 59.4  | 0.6 | 6350 | 80  | 0.26  | 0.08 | 1   |
| 10748390 | 186.6 | 0.4 | 4780 | 50  | 0.31  | 0.05 | 9   |
| 10794087 | 58.0  | 0.4 | 5721 | 50  | 0.25  | 0.08 | 5   |
| 10864656 | 18.6  | 0.5 | 4995 | 78  | -0.07 | 0.1  | 1   |
| 10875245 | 86.4  | 0.4 | 5851 | 75  | 0.27  | 0.1  | 1   |
| 10963065 | 103.2 | 0.6 | 6104 | 74  | -0.20 | 0.1  | 1   |
| 11127479 | 91.6  | 0.6 | 5998 | 57  | -0.20 | 0.3  | 4   |
| 11133306 | 107.5 | 0.5 | 5982 | 82  | -0.02 | 0.1  | 1   |
| 11250587 | 74.0  | 0.6 | 5862 | 97  | 0.27  | 0.11 | 1   |
| 11295426 | 101.5 | 0.4 | 5793 | 74  | 0.12  | 0.07 | 1   |
| 11337566 | 49.6  | 0.5 | 6467 | 173 | -0.10 | 0.3  | 3   |
| 11401755 | 67.8  | 0.5 | 5911 | 66  | -0.20 | 0.06 | 1   |
| 11446443 | 141.2 | 0.4 | 5850 | 50  | -0.15 | 0.1  | 1   |
| 11512246 | 73.4  | 0.3 | 5828 | 100 | -0.05 | 0.1  | 1   |
| 11600889 | 131.8 | 0.5 | 5476 | 75  | 0.33  | 0.07 | 6   |
| 11623629 | 161.1 | 0.4 | 5564 | 50  | -0.14 | 0.08 | 5   |
| 11758544 | 78.2  | 0.3 | 6287 | 169 | -0.27 | 0.3  | 3   |
| 11807274 | 74.9  | 0.7 | 6225 | 75  | 0.00  | 0.08 | 1   |
| 11853905 | 74.4  | 0.3 | 5781 | 76  | 0.09  | 0.1  | 1   |
| 11904151 | 117.9 | 0.4 | 5647 | 74  | -0.15 | 0.1  | 1   |
| 12004971 | 71.3  | 0.3 | 6520 | 178 | 0.04  | 0.3  | 3   |
| 12068975 | 106.8 | 0.6 | 6004 | 102 | -0.38 | 0.1  | 1   |
| 12314973 | 76.3  | 1.3 | 6215 | 89  | 0.28  | 0.1  | 1   |

The large frequency separations ( $\Delta\nu$ ) are from this work, while the spectroscopic parameters ( $T_{\text{eff}}$  and  $[\text{Fe}/\text{H}]$ ) have been found in the literature. The  $\sigma$ -columns give the  $1\sigma$  uncertainties. For references for the spectroscopic values, see the papers listed in the Ref. column and references therein (K15 refers to Hans Kjeldsen et al. (in prep.)).

### Supplementary References:

- [1] Huber, D. *et al.* Fundamental Properties of Kepler Planet-candidate Host Stars using Asteroseismology. *ApJ* **767**, 127 (2013).
- [2] Silva Aguirre, V. *et al.* Ages and fundamental properties of Kepler exoplanet host stars from asteroseismology. *MNRAS* **452**, 2127–2148 (2015).
- [3] Huber, D. *et al.* Revised Stellar Properties of Kepler Targets for the Quarter 1-16 Transit Detection Run. *ApJS* **211**, 2 (2014).
- [4] Chaplin, W. J. *et al.* Asteroseismic Fundamental Properties of Solar-type Stars Observed by the NASA Kepler Mission. *ApJS* **210**, 1 (2014).
- [5] Buchhave, L. A. *et al.* An abundance of small exoplanets around stars with a wide range of metallicities. *Nature* **486**, 375–377 (2012).
- [6] Marcy, G. W. *et al.* Masses, Radii, and Orbits of Small Kepler Planets: The Transition from Gaseous to Rocky Planets. *ApJS* **210**, 20 (2014).
- [7] Rowe, J. F. *et al.* Validation of Kepler’s Multiple Planet Candidates. III. Light Curve Analysis and Announcement of Hundreds of New Multi-planet Systems. *ApJ* **784**, 45 (2014).
- [8] Everett, M. E. *et al.* High-Resolution Multi-Band Imaging for Validation and Characterization of Small Kepler Planets. *AJ* **149**, 55 (2015).
- [9] Bakos, G. Á. *et al.* HAT-P-11b: A Super-Neptune Planet Transiting a Bright K Star in the Kepler Field. *ApJ* **710**, 1724–1745 (2010).
